# Supplementary material for: Geometry-Aware Score Distillation via 3D Consistent Noising and Gradient Consistency Modeling
Source: arXiv:2406.16695 source file (2024-07-01)
Supplement: Supplementary file 1 [file 8_suppl.tex]

% \section{Appendix / supplemental material}

% Optionally include supplemental material (complete proofs, additional experiments and plots) in appendix.
% All such materials \textbf{SHOULD be included in the main submission.}

% \begin{center}
% 	\textbf{\Large Appendix}
% \end{center}

% \input{Suppl_Writing/0_summary}
% \input{Suppl_Writing/1_detail}
% \input{Suppl_Writing/2_more_details}
% \input{Suppl_Writing/3_analysis}
% \newpage
% \input{Suppl_Writing/4_qual}
% \newpage
% \input{Suppl_Writing/5_others}
